# Supplementary material for: Autonomous Diffractometry Enabled by Visual Reinforcement Learning
Source: arXiv:2604.11773 source file (2026-04-13)
Supplement: Supplementary file 2 [file input_supplementary_10.tex]

% Experimental control setup
% empty (just figure)
