# Supplementary material for: Autonomous Diffractometry Enabled by Visual Reinforcement Learning
Source: arXiv:2604.11773 source file (2026-04-13)
Supplement: Supplementary file 3 [file input_supplementary_2.tex]

% Influence of angular solution tolerance and action step size
% empty (just figure)
